# Supplementary material for: Steady-state theory of interdigitated array of electrodes in confined spaces: Case of pure diffusion and reversible electrode reactions
Source: arXiv:1903.02727 source file (2019-03-07)
Supplement: Supplementary file 1 [file text-additional_definitions.tex]

% !TeX root = article
% !TeX encoding = utf8
% !TeX spellcheck = en_US

\section{Jacobian elliptic functions}
\label{elipticas}

In this section \emph{jacobian elliptic functions} are introduced briefly
by using the inverse function $\arcsn()$,
in the same way as $\sin()$ can be introduced from its inverse $\arcsin()$.
Here only a few aspects of jacobian elliptic functions are presented,
those which are considered most relevant for the development of this report.

The complex function $\bm{u} = \arcsn(\bm{v},k)$ with $0 < k < 1$ and $\bm{u},\bm{v} \in \mathds{C}$ \cite[Remark of Example 5.6.8]{Ablowitz:2003:apr}, \cite[\S2.5]{Driscoll2002}, \cite[\S VI.3 Eq. (13)]{Nehari1952}, \cite[{Eq. (\dlmf[E]{22.15.}{12})}]{dlmf}
\begin{equation}
	\bm{u} = \arcsn(\bm{v},k) 
	= \int_{0}^{\bm{v}} \frac{\ud{\bm{w}}}{(1+k\bm{w})^{1/2} (1+\bm{w})^{1/2} (1-\bm{w})^{1/2} (1-k\bm{w})^{1/2}}
\end{equation}
is an odd function
\begin{equation}
	\label{elipticas:eqn:arcsn:odd}
	\arcsn(-\bm{v},k) = -\arcsn(\bm{v},k)
\end{equation}
that corresponds to a case of Schwarz-Christoffel transformation, which maps the real line of the complex domain $\bm{v}$ into the quadrilateral of vertices $(\pm K(k), 0)$ and $(\pm K(k), K'(k))$ in the complex domain $\bm{u}$, and conformally\footnote{a transformation is said to be conformal if it transforms two intersecting curves by preserving their intersection angle. According to \cite[Theorem 5.2.1]{Ablowitz:2003:apr}, \cite[\S V.1 pp. 149-150]{Nehari1952}, \cite[Theorem 5.12]{Olver2016} any complex function that has complex derivative (a.k.a. holomorphic) is a conformal transformation at every point where its derivative is non-zero.} maps the upper half-plane of $\bm{v}$ into the interior of this quadrilateral in $\bm{u}$ \cite[Fig. 5.6.11]{Ablowitz:2003:apr}, \cite[Figs. 2.11, 4.7]{Driscoll2002}, \cite[\S VI.3 Fig. 34]{Nehari1952}. The function $\bm{u} = \arcsn(\bm{v},k)$ produces the following important values on the quadrilateral \cite[Remark of Example 5.6.8]{Ablowitz:2003:apr}, \cite[\S2.5, \S4.3]{Driscoll2002}, \cite[\S VI.3 Eq. (14)]{Nehari1952}, \cite[{Table \dlmf[T]{22.5.}{1}}]{dlmf}
\begin{subequations}
	\label{elipticas:eqn:arcsn:values}
	\begin{align}
		0 &= \arcsn(0,k)
		\\
		\label{idae:eqn:K}
		\pm K(k) &= \arcsn(\pm 1,k) 
		\\
		\pm K(k) + \bm{i} K'(k) &= \arcsn(\pm 1/k,k)
		\\
		\bm{i} K'(k) &= \arcsn(\bm{\infty},k)
	\end{align}
\end{subequations}

The special function $K(k) = \arcsn(1,k)$ is known as the \emph{complete elliptic integral of the first kind} given in terms of the \emph{modulus}\footnote{in some texts the parameter $m=k^{2}$ is used instead of the modulus $k$.} $k$, and its associated function $K'(k) = K(k')$ is given in terms of the \emph{complemetary modulus} $k' = \sqrt{1-k^{2}}$ \cite[Example 5.6.8]{Ablowitz:2003:apr}, \cite[\S2.5]{Driscoll2002}, \cite[\S VI.3 Eqs. (19)--(21)]{Nehari1952} \cite[\S\dlmf{22.}{1}]{dlmf}. Both functions $K(k)$ and $K'(k)$ are also related through another special function $q = Q(k)$ known as the \emph{nome function} \cite[\S VI.3 Eq. (16)]{Nehari1952}, \cite[{Eq. (\dlmf[E]{22.2.}{1})}]{dlmf}
\begin{equation}
	\label{elipticas:eqn:nomo}
	\frac{\ln Q(k)}{-\pi} = \frac{-\pi}{\ln Q(k')} = \frac{K'(k)}{K(k)}
\end{equation}
where $K'(k) = K(k')$ was also used to obtain this relation.

The jacobian elliptic function $\bm{v} = \sn(\bm{u},k)$ is a double-periodic function \cite[Eq. 5.6.12]{Ablowitz:2003:apr}, \cite[\S VI.3 Eq. (22)]{Nehari1952}, \cite[{Tables \dlmf[T]{22.4.}{1} and \dlmf[T]{22.4.}{2}}]{dlmf}
\begin{equation}
	\label{elipticas:eqn:sn:period}
	\sn(\bm{u},k) = \sn(\bm{u} + n 4K(k) + \bm{i} m 2K'(k),k)\quad n,m\in\mathds{Z}
\end{equation}
which satisfies the following half-period and quarter-period properties \cite[{Table \dlmf[T]{22.4.}{3}}]{dlmf}
\begin{subequations}
	\label{elipticas:eqn:sn:periods}
	\begin{align}
	\sn(\bm{u} - 2K(k),k) = \sn(\bm{u} + 2K(k),k) &= -\sn(\bm{u},k) 
	\label{elipticas:eqn:sn:half} \\
	\sn(\bm{u} - 3K(k),k) = \sn(\bm{u} + K(k),k) &= \phantom{-} \cd(\bm{u},k) 
	\label{elipticas:eqn:sn:quarter}
	\end{align}
\end{subequations}
%where $\cd = \cn/\dn$. 
and presents odd symmetry
\begin{equation}
	\label{elipticas:eqn:sn:odd}
	\sn(-\bm{u},k) = -\sn(\bm{u},k)
\end{equation}
This function corresponds to the inverse function of  $\bm{u} = \arcsn(\bm{v},k)$, and it can be regarded as a generalization of the circular funcion $\sin()$ to the elliptical case. 

Similarly, the jacobian elliptic function $\cn()$, corresponds to the elliptic generalization of the circular function $\cos()$ which satisfies \cite[\S VI.3 Eq. (17)]{Nehari1952}, \cite[{Eq. (\dlmf[E]{22.6.}{1})}]{dlmf}
\begin{equation}
	\sn(\bm{u},k)^{2} + \cn(\bm{u},k)^{2} = 1
\end{equation}
and the jacobian elliptic function $\dn()$ relates with $\sn()$ through the identity \cite[\S VI.3 Eq. (18)]{Nehari1952}, \cite[{Eq. (\dlmf[E]{22.6.}{1})}]{dlmf}
\begin{equation}
	k^{2} \sn(\bm{u},k)^{2} + \dn(\bm{u},k)^{2} = 1
\end{equation}
These are the most elementary jacobian elliptic functions, and the most basic relations among them.

Also there are remaining nine subsidiary jacobian elliptic functions that can be obtained from the three elementary functions $\sn()$, $\cn()$ and $\dn()$ according to \cite[{Eq. (\dlmf[E]{22.2.}{10})}]{dlmf}
\begin{equation}
	\pq(\bm{u},k) = \frac{\pr(\bm{u},k)}{\qr(\bm{u},k)}
\end{equation}
where p,q,r $\in$ \{s,c,d,n\} and $\pp(\bm{u},k)=1$. More relations and properties among all these functions can be found in \cite[\S\dlmf{22}{}]{dlmf}.
